# Supplementary material for: How to Measure Human-AI Prediction Accuracy in Explainable AI Systems
Source: arXiv:2409.00069 source file (2024-08-23)
Supplement: Supplementary file 1 [file 2_PredictionCounts.pdf]

Predict 1: NONE

| | A | B | C | D | E | F | G | H | I |
|---|---|---|---|---|---|---|---|---|---|
| 1 | | | 1 | 2 | X | | | | |
| 2 | | | O | 3 | 4 | 1 | | | |
| 3 | | | | | | | | | |
| 4 | | | | | | | | | |

Predict 1: STT Only

| | A | B | C | D | E | F | G | H | I |
|---|---|---|---|---|---|---|---|---|---|
| 1 | | | | 1 | X | 1 | | | |
| 2 | | | O | 3 | 1 | 1 | | | |
| 3 | | | 1 | | | | | | |
| 4 | | | | | | | | | |

Predict 1: STT & OTB

| | A | B | C | D | E | F | G | H | I |
|---|---|---|---|---|---|---|---|---|---|
| 1 | | | | 1 | X | 2 | | | |
| 2 | | 1 | O | 2 | 3 | 1 | | | |
| 3 | | | | 1 | 1 | | | | |
| 4 | | | | | | | | | |

Predict 1: STT & BTW

| | A | B | C | D | E | F | G | H | I |
|---|---|---|---|---|---|---|---|---|---|
| 1 | | | | 2 | X | 2 | | | |
| 2 | | | O | 2 | 2 | 3 | | | |
| 3 | | | | | | | | | |
| 4 | | | | | | | | | |

Predict 1: BTW Only

| | A | B | C | D | E | F | G | H | I |
|---|---|---|---|---|---|---|---|---|---|
| 1 | | | | 1 | X | 2 | | | |
| 2 | | | O | 2 | 2 | 1 | | | |
| 3 | | | 1 | | | | 1 | | |
| 4 | | | | | | | | | |

Predict 1: OTB Only

| | A | B | C | D | E | F | G | H | I |
|---|---|---|---|---|---|---|---|---|---|
| 1 | | | | | X | 1 | | | |
| 2 | | | O | 4 | 2 | 1 | | | |
| 3 | | | | | 1 | | | | |
| 4 | | | | | 1 | | | | |

Predict 1: OTB & BTW

| | A | B | C | D | E | F | G | H | I |
|---|---|---|---|---|---|---|---|---|---|
| 1 | | | 1 | | X | 2 | 1 | | |
| 2 | | | O | 2 | 7 | | | | |
| 3 | | | | | | | | | |
| 4 | | | | | | | | | |

Predict 1: ALL

| | A | B | C | D | E | F | G | H | I |
|---|---|---|---|---|---|---|---|---|---|
| 1 | | | | 4 | X | | | | |
| 2 | | | O | 2 | 3 | 2 | | | |
| 3 | | | | | | | | | |
| 4 | | | | | | | | | |

### Predict 2: NONE

| | A | B | C | D | E | F | G | H | I |
|---|---|---|---|---|---|---|---|---|---|
| 1 | | | | | X | | | | |
| 2 | | | O | | 1 | X | | | |
| 3 | | | | O | | | 8 | | |
| 4 | | | | | 2 | | | | |

### Move 2: BTW

| | A | B | C | D | E | F | G | H | I |
|---|---|---|---|---|---|---|---|---|---|
| 1 | | | | 1 | X | 2 | | | |
| 2 | | | O | 2 | 2 | X | | | |
| 3 | | | 1 | O | | | 1 | | |
| 4 | | | | | | | | | |

### Move 2: STT

| | A | B | C | D | E | F | G | H | I |
|---|---|---|---|---|---|---|---|---|---|
| 1 | | | | | X | | | | |
| 2 | | | O | | 3 | X | 1 | | |
| 3 | | | | O | | | 4 | | |
| 4 | | | | | | | | | |

### Move 2: OTB

| | A | B | C | D | E | F | G | H | I |
|---|---|---|---|---|---|---|---|---|---|
| 1 | | | | | X | | | | |
| 2 | | | O | 1 | 1 | X | | | |
| 3 | | | | O | | | 7 | | |
| 4 | | | | | 1 | | | | |

### Move 2: STT+OTB

| | A | B | C | D | E | F | G | H | I |
|---|---|---|---|---|---|---|---|---|---|
| 1 | | | | | X | | 1 | | |
| 2 | | | O | | 1 | X | | | |
| 3 | | | | O | 1 | | 9 | | |
| 4 | | | | | | | | | |

### Move 2: OTB+BTW

| | A | B | C | D | E | F | G | H | I |
|---|---|---|---|---|---|---|---|---|---|
| 1 | | | | | X | | 1 | | |
| 2 | | | O | | 2 | X | | | |
| 3 | | | | O | 2 | 1 | 7 | | |
| 4 | | | | | | | | | |

### Move 2: STT+BTW

| | A | B | C | D | E | F | G | H | I |
|---|---|---|---|---|---|---|---|---|---|
| 1 | | | | | X | | | | |
| 2 | | | O | 1 | 2 | X | 1 | | |
| 3 | | | | O | | | 5 | | |
| 4 | | | | | 2 | | | | |

### Move 2: ALL

| | A | B | C | D | E | F | G | H | I |
|---|---|---|---|---|---|---|---|---|---|
| 1 | | | | | X | | | | |
| 2 | | | O | 1 | | X | | | |
| 3 | | | | O | 1 | | 6 | | |
| 4 | | | | | 3 | | | | |

Predict 3: NONE

| | A | B | C | D | E | F | G | H | I |
|---|---|---|---|---|---|---|---|---|---|
| 1 | | | | | X | | | | |
| 2 | | | O | X | 5 | X | | | |
| 3 | | | 4 | O | 1 | | 1 | | |
| 4 | | | O | | | | | | |

Predict 3: BTW

| | A | B | C | D | E | F | G | H | I |
|---|---|---|---|---|---|---|---|---|---|
| 1 | | | | | X | | | | |
| 2 | | | O | X | 7 | X | | | |
| 3 | | | 3 | O | | | | | |
| 4 | | | O | | | | | | |

Predict 3: STT

| | A | B | C | D | E | F | G | H | I |
|---|---|---|---|---|---|---|---|---|---|
| 1 | | | 1 | | X | 1 | | | |
| 2 | | | O | X | 1 | X | 1 | | |
| 3 | | | 4 | O | | | | | |
| 4 | | | O | | | | | | |

Predict 3: OTB

| | A | B | C | D | E | F | G | H | I |
|---|---|---|---|---|---|---|---|---|---|
| 1 | | | 1 | | X | | | | |
| 2 | | | O | X | 6 | X | | | |
| 3 | | | 2 | O | | | | | |
| 4 | | | O | | 1 | | | | |

Predict 3: STT+OTB

| | A | B | C | D | E | F | G | H | I |
|---|---|---|---|---|---|---|---|---|---|
| 1 | | | | | X | | | | |
| 2 | | | O | X | 5 | X | 1 | | |
| 3 | | | 2 | O | 3 | | | | |
| 4 | | | O | | 1 | | | | |

Predict 3: OTB+BTW

| | A | B | C | D | E | F | G | H | I |
|---|---|---|---|---|---|---|---|---|---|
| 1 | | | 1 | | X | | | | |
| 2 | | | O | X | 7 | X | | | |
| 3 | | | 3 | O | 2 | | | | |
| 4 | | | O | | | | | | |

Predict 3: STT+BTW

| | A | B | C | D | E | F | G | H | I |
|---|---|---|---|---|---|---|---|---|---|
| 1 | | | | 1 | X | | | | |
| 2 | | | O | X | 3 | X | 1 | | |
| 3 | | | 4 | O | 2 | | | | |
| 4 | | | O | | | | | | |

Predict 3: ALL

| | A | B | C | D | E | F | G | H | I |
|---|---|---|---|---|---|---|---|---|---|
| 1 | | | | | X | | | | |
| 2 | | | O | X | 4 | X | | | |
| 3 | | | 4 | O | 2 | | 1 | | |
| 4 | | | O | | | | | | |

Predict 4: NONE

| | A | B | C | D | E | F | G | H | I |
|---|---|---|---|---|---|---|---|---|---|
| 1 | | | | | X | | | | |
| 2 | | | O | X | 10 | X | X | 1 | |
| 3 | | | | O | O | O | | | |
| 4 | | | O | | | | | | |

Predict 4: BTW

| | A | B | C | D | E | F | G | H | I |
|---|---|---|---|---|---|---|---|---|---|
| 1 | | | | | 1 | | | | |
| 2 | | | O | X | 9 | X | X | | |
| 3 | | | | O | O | O | | | |
| 4 | | | O | | | | | | |

Predict 4: STT

| | A | B | C | D | E | F | G | H | I |
|---|---|---|---|---|---|---|---|---|---|
| 1 | | | | | X | | | | |
| 2 | | | O | X | 7 | X | X | | |
| 3 | | | | O | O | O | 1 | | |
| 4 | | | O | | | | | | |

Predict 4: OTB

| | A | B | C | D | E | F | G | H | I |
|---|---|---|---|---|---|---|---|---|---|
| 1 | | | | | X | | | | |
| 2 | | | O | X | 10 | X | X | | |
| 3 | | | | O | O | O | | | |
| 4 | | | O | | | | | | |

Predict 4: STT+OTB

| | A | B | C | D | E | F | G | H | I |
|---|---|---|---|---|---|---|---|---|---|
| 1 | | | | | X | | | | |
| 2 | | | O | X | 11 | X | X | 1 | |
| 3 | | | | O | O | O | | | |
| 4 | | | O | | | | | | |

Predict 4: OTB+BTW

| | A | B | C | D | E | F | G | H | I |
|---|---|---|---|---|---|---|---|---|---|
| 1 | | | | | X | | | | |
| 2 | | | O | X | 13 | X | X | | |
| 3 | | | | O | O | O | | | |
| 4 | | | O | | | | | | |

Predict 4: STT+BTW

| | A | B | C | D | E | F | G | H | I |
|---|---|---|---|---|---|---|---|---|---|
| 1 | | | | | X | | | | |
| 2 | | | O | X | 9 | X | X | | |
| 3 | | | | O | O | O | 2 | | |
| 4 | | | O | | | | | | |

Predict 4: ALL

| | A | B | C | D | E | F | G | H | I |
|---|---|---|---|---|---|---|---|---|---|
| 1 | | | | | X | | | | |
| 2 | | | O | X | 8 | X | X | | |
| 3 | | | 1 | O | O | O | 1 | | |
| 4 | | | O | | 1 | | | | |

Prediction 1: Aggregate

| | A | B | C | D | E | F | G | H | I |
|---|---|---|---|---|---|---|---|---|---|
| 1 | | | 2 | 11 | X | 10 | 1 | | |
| 2 | | 1 | O | 20 | 24 | 10 | | | |
| 3 | | | 2 | 1 | 2 | | 1 | | |
| 4 | | | | | 1 | | | | |

Prediction 1: Comprehensive

| | A | B | C | D | E | F | G | H | I |
|---|---|---|---|---|---|---|---|---|---|
| 1 | | | 1 | 7 | X | 5 | | | |
| 2 | | 1 | O | 10 | 8 | 4 | | | |
| 3 | | | 1 | | 1 | | 1 | | |
| 4 | | | | | | | | | |

Prediction 1: Selective

| | A | B | C | D | E | F | G | H | I |
|---|---|---|---|---|---|---|---|---|---|
| 1 | | | 1 | 4 | X | 5 | 1 | | |
| 2 | | | O | 10 | 16 | 6 | | | |
| 3 | | | 1 | 1 | 1 | | | | |
| 4 | | | | | 1 | | | | |

Prediction 2: Aggregate

| | A | B | C | D | E | F | G | H | I |
|---|---|---|---|---|---|---|---|---|---|
| 1 | | | | | X | | 2 | | |
| 2 | | | O | 3 | 11 | X | 3 | | |
| 3 | | | | O | 4 | 1 | 53 | | |
| 4 | | | | | 9 | | | | |

Prediction 2: Comprehensive

| | A | B | C | D | E | F | G | H | I |
|---|---|---|---|---|---|---|---|---|---|
| 1 | | | | | X | | 1 | | |
| 2 | | | O | 1 | 6 | X | | | |
| 3 | | | | O | | 1 | 28 | | |
| 4 | | | | | 2 | | | | |

Prediction 2: Selective

| | A | B | C | D | E | F | G | H | I |
|---|---|---|---|---|---|---|---|---|---|
| 1 | | | | | X | | 1 | | |
| 2 | | | O | 2 | 5 | X | 3 | | |
| 3 | | | | O | 4 | | 25 | | |
| 4 | | | | | 7 | | | | |

Prediction 3: Aggregate

| | A | B | C | D | E | F | G | H | I |
|---|---|---|---|---|---|---|---|---|---|
| 1 | | | 3 | 1 | X | 1 | | | |
| 2 | | | O | X | 38 | X | 3 | | |
| 3 | | | 26 | O | 10 | | 2 | | |
| 4 | | | O | | 2 | | | | |

Prediction 3: Comprehensive

| | A | B | C | D | E | F | G | H | I |
|---|---|---|---|---|---|---|---|---|---|
| 1 | | | | | X | | | | |
| 2 | | | O | X | 18 | X | 2 | | |
| 3 | | | 15 | O | 3 | | | | |
| 4 | | | O | | 1 | | | | |

Prediction 3: Selective

| | A | B | C | D | E | F | G | H | I |
|---|---|---|---|---|---|---|---|---|---|
| 1 | | | 3 | 1 | X | 1 | | | |
| 2 | | | O | X | 20 | X | 1 | | |
| 3 | | | 11 | O | 7 | | 2 | | |
| 4 | | | O | | 1 | | | | |

Prediction 4: Aggregate

| | A | B | C | D | E | F | G | H | I |
|---|---|---|---|---|---|---|---|---|---|
| 1 | | | | | X | | | | |
| 2 | | | O | X | 77 | X | X | 2 | |
| 3 | | | 1 | O | O | | 4 | | |
| 4 | | | O | | 1 | | | | |

Prediction 4: Comprehensive

| | A | B | C | D | E | F | G | H | I |
|---|---|---|---|---|---|---|---|---|---|
| 1 | | | | | X | | | | |
| 2 | | | O | X | 37 | X | X | 2 | |
| 3 | | | | O | O | | | | |
| 4 | | | O | | | | | | |

Prediction 4: Selective

| | A | B | C | D | E | F | G | H | I |
|---|---|---|---|---|---|---|---|---|---|
| 1 | | | | | **1** | | | | |
| 2 | | | O | X | 40 | X | X | | |
| 3 | | | 1 | O | O | | 4 | | |
| 4 | | | O | | 1 | | | | |
